# Supplementary material for: Data Poisoning to Fake a Nash Equilibrium in Markov Games
Source: arXiv:2306.08041 source file (2024-06-18)
Supplement: Supplementary file 1 [file appendix.tex]

\onecolumn
\section{Supplementary Material}

\subsection{Proof of Proposition~\ref{prop:unp} and Theorem~\ref{thm:unpm}}
We show that for zero-sum games, strict MPEs are MPEs and they are unique. We use the following definition of MPE and strict MPE for zero-sum games rewritten in terms of $\text{Q}$ functions. Proposition~\ref{prop:unp} is a special case of Theorem~\ref{thm:unpm} with $H = \left| \mS \right| = 1$.

\begin{df}  \label{df:zsmpd} 
(Markov Perfect Equilibrium for Zero-sum Games$) \pidag$ is a MPE if for each $h \in \left[H\right], s \in \mS$,
\begin{align}
\Qh^{\pidag}\left(s, \pidagh\left(s\right)\right) &\geq \Qh^{\pidag}\left(s, \left(a_{1}, \pidaghb\left(s\right)\right)\right), \forall\; a_{1} \neq \pidagha\left(s\right), \label{eq:rabr}
\\ \Qh^{\pidag}\left(s, \pidagh\left(s\right)\right) &\leq \Qh^{\pidag}\left(s, \left(\pidagha\left(s\right), a_{2}\right)\right), \forall\; a_{2} \neq \pidaghb\left(s\right). \label{eq:rbbr}
\end{align}\end{df}
\begin{df}  \label{df:zssmpd} 
(Strict Markov Perfect Equilibrium for Zero-sum Games$) \pidag$ is a strict MPE if for each $h \in \left[H\right], s \in \mS$,
\begin{align}
\Qh^{\pidag}\left(s, \pidagh\left(s\right)\right) &> \Qh^{\pidag}\left(s, \left(a_{1}, \pidaghb\left(s\right)\right)\right), \forall\; a_{1} \neq \pidagha\left(s\right), \label{eq:abr}
\\ \Qh^{\pidag}\left(s, \pidagh\left(s\right)\right) &< \Qh^{\pidag}\left(s, \left(\pidagha\left(s\right), a_{2}\right)\right), \forall\; a_{2} \neq \pidaghb\left(s\right). \label{eq:bbr}
\end{align}\end{df}
\begin{proof}  \label{proof:unpmpf} 
Fix a period $h \in \left[H\right]$, and assume in periods $h + 1, h + 2, ..., H, \pidag$ is the unique NE in every state $s \in \mS$. This is vacuously true in period $H$.
\\* First, $\pidagh\left(s\right)$ is a NE since ~\eqref{eq:abr} implies ~\eqref{eq:rabr} and ~\eqref{eq:bbr} implies ~\eqref{eq:rbbr}.
\\* Now, for a contradiction, assume $\left(a^{'}_{1}, a^{'}_{2}\right) \neq \pidagh\left(s\right)$ is another NE in the stage game in period $h$ in some state $s \in \mS$, then,
\begin{align}
\Qh^{\pidag}\left(s, \left(a^{'}_{1}, a^{'}_{2}\right)\right) &\geq \Qh^{\pidag}\left(s, \left(\pidagha\left(s\right), a^{'}_{2}\right)\right), \label{eq:qbp}
\\ \Qh^{\pidag}\left(s, \left(a^{'}_{1}, a^{'}_{2}\right)\right) &\leq \Qh^{\pidag}\left(s, \left(a^{'}_{1}, \pidaghb\left(s\right)\right)\right). \label{eq:qap}
\end{align}
From the strict MPE conditions,
\begin{align}
\Qh^{\pidag}\left(s, \pidagh\left(s\right)\right) &\stackrel{~\eqref{eq:abr}}{>} \Qh^{\pidag}\left(s, \left(\pidagha\left(s\right), a^{'}_{2}\right)\right), \label{eq:nqbp}
\\ \Qh^{\pidag}\left(s, \pidagh\left(s\right)\right) &\stackrel{~\eqref{eq:bbr}}{<} \Qh^{\pidag}\left(s, \left(a^{'}_{1}, \pidaghb\left(s\right)\right)\right). \label{eq:nqap}
\end{align}
Combine the above inequalities, we get,
\begin{align}
\Qh^{\pidag}\left(s, \pidagh\left(s\right)\right) &\stackrel{~\eqref{eq:qbp},~\eqref{eq:nqbp}}{>} \Qh^{\pidag}\left(s, \left(a^{'}_{1}, a^{'}_{2}\right)\right),
\\ \Qh^{\pidag}\left(s, \pidagh\left(s\right)\right) &\stackrel{~\eqref{eq:qap},~\eqref{eq:nqap}}{<} \Qh^{\pidag}\left(s, \left(a^{'}_{1}, a^{'}_{2}\right)\right),
\end{align}
which is a contradiction.
\\* Therefore, $\pidag$ is the unique NE in period $h$, state $s$. Since $h$ and $s$ are arbitrary, $\pidag$ is the unique MPE.

\end{proof}

\subsection{Proof of Proposition~\ref{prop:rplp} and Theorem~\ref{thm:rplpm}}
We first write out the complete optimization problem for ~\eqref{eq:emlclpm} in Example~\ref{eg:mlclpm}, then we show that the optimization is a relaxation by showing for any $Q^{\pidag} \in \left[\Ql^{\pidag}, \Qu^{\pidag}\right]$ elememtwise, $\pidag$ is a strict MPE, and as a result Theorem~\ref{thm:unpm} implies its uniqueness. The proof that the problem can be converted into a linear program is similar to LP conversions in ~\citep{wu2022reward}. We do not write out the complete LP, and instead we show that each constraint can be converted into a linear constraint. Theorem~\ref{thm:rplpm} is a special case of ~\eqref{eq:emlclpm} with given $\Ql^{\pidag}$ and $\Qu^{\pidag}$ that are not derived from the rewards and transitions, and Proposition~\ref{prop:rplp} is a special case of Theorem~\ref{thm:rplpm} when $H = \left| \mS \right| = 1$.

\begin{align}
\displaystyle\min_{\rdag \in \left[0, 1\right]^{H K}} & \displaystyle\sum_{k=1}^{K} \displaystyle\sum_{h=1}^{H} \left| \rdagkh - \rkh \right|\nonumber
\\ \text{\;subject to\;} & \Rh\left(s, \textbf{a}\right) = \dfrac{\displaystyle\sum_{k=1}^{K} \displaystyle\sum_{h=1}^{H} \rdagkh \mathbb{I}_{\left\{\skh = s, \akh = \textbf{a}\right\}}}{\displaystyle\max\left\{\Nh\left(s, \textbf{a}\right), 1\right\}}, \hspace{2em} \forall\; h \in \left[H\right], s \in \mS, \textbf{a} \in \mA, \label{eq:srhat}
\\ & \Ph\left(s' | s, \textbf{a}\right) = \dfrac{\displaystyle\sum_{k=1}^{K} \mathbb{I}_{\left\{\skhh = s', \skh = s, \akh = \textbf{a}\right\}}}{\Nh\left(s, \textbf{a}\right)} \text{\;or\;} \dfrac{1}{\left| \mS \right|} \text{\;if\;} \Nh\left(s, \textbf{a}\right) = 0, \hspace{2em} \forall\; h \in \left[H\right], s \in \mS, \textbf{a} \in \mA,  \label{eq:sphat}
\\ & \Qlh^{\pidag}\left(s, \textbf{a}\right) = \displaystyle\min_{R \in \mCRih\left(s, \textbf{a}\right)} R + \displaystyle\min_{P \in \mCPh\left(s, \textbf{a}\right)} \displaystyle\sum_{s' \in \mS} P\left(s'\right) \Qlhh^{\pidag}\left(s', \pidaghh\left(s'\right)\right), \hspace{2em} \forall\; h \in \left[H\right], s \in \mS, \textbf{a} \in \mA, \label{eq:qlh}
\\ & \Quh^{\pidag}\left(s, \textbf{a}\right) = \displaystyle\max_{R \in \mCRih\left(s, \textbf{a}\right)} R + \displaystyle\max_{P \in \mCPh\left(s, \textbf{a}\right)} \displaystyle\sum_{s' \in \mS} P\left(s'\right) \Quhh^{\pidag}\left(s', \pidaghh\left(s'\right)\right), \hspace{2em} \forall\; h \in \left[H\right], s \in \mS, \textbf{a} \in \mA,\label{eq:quh}
\\ & \QlHH^{\pidag}\left(s, \textbf{a}\right) = \QuHH^{\pidag}\left(s, \textbf{a}\right) = 0, \hspace{2em} \forall\; s \in \mS, \textbf{a} \in \mA,\nonumber
\\ & \Qlh^{\pidag}\left(s, \pidagh\left(s\right)\right) \geq \Quh^{\pidag}\left(s, \left(a_{1}, \pidaghb\left(s\right)\right)\right) + \iota, \hspace{2em} \forall\; h \in \left[H\right], s \in \mS, a_{1} \neq \pidagha\left(s\right),\label{eq:lpqa}
\\ & \Quh^{\pidag}\left(s, \pidagh\left(s\right)\right) \leq \Qlh^{\pidag}\left(s, \left(\pidagha\left(s\right), a_{2}\right)\right) - \iota, \hspace{2em} \forall\; h \in \left[H\right], s \in \mS, a_{2} \neq \pidaghb\left(s\right).\label{eq:lpqb}
\end{align}
Since we evaluate the $\Ql$ and $\Qu$ functions on the policy $\pidag$, we add superscript $\pidag$ on $\Ql$ and $\Qu$ inside the optimization for clarity.

\begin{proof}  \label{proof:rplpmpf} 
Take any $R \in \mCR$ and $P \in \mCP$, due to the definition of $\Ql^{\pidag}$ and $\Qu^{\pidag}$, which are replicated in ~\eqref{eq:qlh} and ~\eqref{eq:quh}, we know that, for each $h \in \left[H\right], s \in \mS, \textbf{a} \in \mA$,
\begin{align}
\Qlh^{\pidag}\left(s, \textbf{a}\right) &\leq \Qh^{\pidag}\left(s, \textbf{a}\right) \leq \Quh^{\pidag}\left(s, \textbf{a}\right). \label{eq:qbtw}
\end{align}
Fix period $h \in \left[H\right]$, and assume in periods $h + 1, h + 2, ..., H, \pidag$ is the Nash equilibrium in every state $s \in \mS$. This is vacuously true in period $H$.
\\* For a fixed $s \in \mS$, for any $a_{1} \neq \pidagha\left(s\right)$,
\begin{align}
\Qh^{\pidag}\left(s, \pidagh\left(s\right)\right) &\stackrel{~\eqref{eq:qbtw}}{\geq} \Qlh^{\pidag}\left(s, \pidagh\left(s\right)\right)\nonumber
\\ &\stackrel{~\eqref{eq:lpqa}}{\geq} \Quh^{\pidag}\left(s, \left(a_{1}, \pidaghb\left(s\right)\right)\right) + \iota\nonumber
\\ &\stackrel{~\eqref{eq:qbtw}}{\geq} \Qh^{\pidag}\left(s, \left(a_{1}, \pidaghb\left(s\right)\right)\right) + \iota, \label{eq:lpqqa}
\end{align}
and for any $a_{2} \neq \pidaghb\left(s\right)$,
\begin{align}
\Qh^{\pidag}\left(s, \pidagh\left(s\right)\right) &\stackrel{~\eqref{eq:qbtw}}{\leq} \Quh^{\pidag}\left(s, \pidagh\left(s\right)\right)\nonumber
\\ &\stackrel{~\eqref{eq:lpqb}}{\leq} \Qlh^{\pidag}\left(s, \left(\pidagha\left(s\right), a_{2}\right)\right) - \iota\nonumber
\\ &\stackrel{~\eqref{eq:qbtw}}{\geq} \Qh^{\pidag}\left(s, \left(\pidaghb\left(s\right), a_{2}\right)\right) - \iota, \label{eq:lpqqb}
\end{align}
~\eqref{eq:lpqqa} and ~\eqref{eq:lpqqb} imply that $\pidagh\left(s\right)$ is the Nash equilibrium in period $h$ state $s$.
\\* Therefore, $Q^{\pidag} \in \bNash\left(\pidag; \iota\right)$, and by Theorem~\ref{thm:unpm}, $\pidag$ is the unique MPE.
\\* Now, to show that the problem can be converted into an LP, we note that ~\eqref{eq:srhat} is linear in $\rdag$, ~\eqref{eq:sphat} is independent of $\rdag$, ~\eqref{eq:lpqa} and ~\eqref{eq:lpqb} are linear in $\Ql$ and $\Qu$. Therefore, we only have to convert ~\eqref{eq:qlh} and ~\eqref{eq:quh}, which define $\Ql$ and $\Qu$ into linear constraints in $\rdag$, in particular, we convert the following linear program, for some $h \in \left[H\right], s \in \mS, \textbf{a} \in \mA$,
\begin{align}
\displaystyle\min_{P} \displaystyle\sum_{s' \in \mS} & P\left(s'\right) \Qlhh^{\pidag}\left(s', \pidaghh\left(s'\right)\right)\nonumber
\\ \text{\;subject to\;} & P\left(s'\right) \leq \Phh\left(s' | s, \textbf{a}\right) + \rhoPh\left(s, \textbf{a}\right), \forall\; s' \in \mS,\nonumber
\\ & P\left(s'\right) \geq \Phh\left(s' | s, \textbf{a}\right) - \rhoP\left(s, \textbf{a}\right), \forall\; s' \in \mS,\nonumber
\\ & \displaystyle\sum_{s' \in \mS} P\left(s'\right) = 1,\nonumber
\\ & P\left(s'\right) \geq 0, \forall\; s' \in \mS,\nonumber
\end{align}
into its dual problem,
\begin{align}
\displaystyle\max_{\underline{u} \in \mathbb{R}^{\mS}, \underline{v} \in \mathbb{R}^{\mS}, \underline{w} \in \mathbb{R}} & \displaystyle\sum_{s' \in \mS} \Phh\left(s' | s, \textbf{a}\right)\left(\underline{u}_{s'} - \underline{v}_{s'}\right) + \rhoPh\left(s, \textbf{a}\right) \left(\underline{u}_{s'} + \underline{v}_{s'}\right) + \underline{w}\nonumber
\\ \text{\;subject to\;} & \underline{u}_{s'} - \underline{v}_{s'} + \underline{w} \geq -\Qlhh^{\pidag}\left(s', \pidaghh\left(s'\right)\right), \forall\; s' \in \mS,\nonumber
\\ & \underline{u}_{s'} \geq 0, \underline{v}_{s'} \geq 0, \forall\; s' \in \mS.\nonumber
\end{align}
Therefore, ~\eqref{eq:qlh} can be rewritten as the following linear constraints,
\begin{align}
\Qlh^{\pidag}\left(s, \textbf{a}\right) &= \Rh\left(s, \textbf{a}\right) - \rhoRh\left(s, \textbf{a}\right) + \displaystyle\sum_{s' \in \mS} \Phh\left(s' | s, \textbf{a}\right)\left(\underline{u}_{s'} - \underline{v}_{s'}\right) + \rhoPh\left(s, \textbf{a}\right) \left(\underline{u}_{s'} + \underline{v}_{s'}\right) + \underline{w},\nonumber
\\ \underline{u}_{s'} - \underline{v}_{s'} + \underline{w} &\geq -\Qlhh^{\pidag}\left(s', \pidaghh\left(s'\right)\right), \forall\; s' \in \mS,\nonumber
\\ \underline{u}_{s'} &\geq 0, \underline{v}_{s'} \geq 0, \forall\; s' \in \mS.\nonumber
\end{align}
The similar dual problem can be written out for the $\Qu$ to replace ~\eqref{eq:quh},
\begin{align}
\Quh^{\pidag}\left(s, \textbf{a}\right) &= \Rh\left(s, \textbf{a}\right) + \rhoRh\left(s, \textbf{a}\right) + \displaystyle\sum_{s' \in \mS} \Phh\left(s' | s, \textbf{a}\right)\left(\overline{u}_{s'} - \overline{v}_{s'}\right) + \rhoPh\left(s, \textbf{a}\right) \left(\overline{u}_{s'} + \overline{v}_{s'}\right) + \overline{w},\nonumber
\\ \overline{u}_{s'} - \overline{v}_{s'} + \overline{w} &\geq \Quhh^{\pidag}\left(s', \pidaghh\left(s'\right)\right), \forall\; s' \in \mS,\nonumber
\\ \overline{u}_{s'} &\geq 0, \overline{v}_{s'} \geq 0, \forall\; s' \in \mS.\nonumber
\end{align}
The linearization of the other $\Ql$ and $\Qu$ constraints are similar.

\end{proof}

\subsection{Proof of Theorem~\ref{thm:rplpf}}
Again, we write the proof for ~\eqref{eq:emlclpm} in Example~\ref{eg:mlclpm}, and Theorem~\ref{thm:rplpf} is a special case with given $\Ql^{\pidag}$ and $\Qu^{\pidag}$ that are not derived from the rewards and transitions. In particular, setting $\rhoQ = \rhoR$ and $\rhoP = 0$ would like to the result stated in Theorem~\ref{thm:rplpf}. We first provide the intuition behind the proofs. The proof is at the end of this subsection.

Suppose the target action profile is $\left(1, 1\right)$ in some state $s$ in period $h$, we show that the target action profile $\left(1, 1\right)$ is the unique NE for any $\Qh\left(s, \cdot\right) \in \left[\Qlh\left(s, \cdot\right), \Quh\left(s, \cdot\right)\right]$ under the following attack,
\begin{align}
\rdagkh &= \begin{cases} -b & \text{\;if\;} \akha \neq \pidagha\left(\skh\right), \akhb = \pidaghb\left(\skh\right) \\ 0 & \text{\;if\;} \akha = \pidagha\left(\skh\right), \akhb = \pidaghb\left(\skh\right) \\ b & \text{\;if\;} \akha = \pidagha\left(\skh\right), \akhb \neq \pidaghb\left(\skh\right) \\ \rkh & \text{\;otherwise\;} \\ \end{cases}. \label{eq:fsatk}
\end{align}
To simplify the notations, we define the bounds on the cumulative $Q$ value in period $h + 1, h + 2, ..., H$ as,
\begin{align}
\Slh &= \displaystyle\sum_{h' = h + 1}^{H} \displaystyle\min_{s' \in \mS} \Qlhp\left(s', \pidaghp\left(s'\right)\right)\nonumber
\\ \Suh &= \displaystyle\sum_{h' = h + 1}^{H} \displaystyle\max_{s' \in \mS} \Quhp\left(s', \pidaghp\left(s'\right)\right)\nonumber
\end{align}
$\Qlh\left(s\right)$ is lower bounded by,

\begin{center} \begin{tabular}{|c|c|c|c|c|c|}
\hline
 $\mAa \setminus \mAb$ &$1$ &$2$ &$...$ &$\left| \mAb \right|$\\ \hline
$1$ &$0 - \rhoRh\left(s, \left(1, 1\right)\right) +  \Slh$ &$b - \rhoRh\left(s, \left(1, 2\right)\right) + \Slh$ &$...$ &$b - \rhoRh\left(s, \left(1, \left| \mAb \right|\right)\right) + \Slh$\\ \hline
$2$ &$-b - \rhoRh\left(s, \left(2, 1\right)\right) +  \Slh$ &? &$...$ &?\\ \hline
$...$ &$...$ &$...$ &$...$ &$...$\\ \hline
$\left| \mAa \right|$ &$- b - \rhoRh\left(s, \left(\left| \mAa \right|, 1\right)\right) +  \Slh$ &? &$...$ &?\\ \hline
\end{tabular} \end{center}
$\Quh\left(s\right)$ is upper bounded by,

\begin{center} \begin{tabular}{|c|c|c|c|c|c|}
\hline
 $\mAa \setminus \mAb$ &$1$ &$2$ &$...$ &$\left| \mAb \right|$\\ \hline
$1$ &$0 + \rhoRh\left(s, \left(1, 1\right)\right) +  \Suh$ &$b + \rhoRh\left(s, \left(1, 2\right)\right) + \Suh$ &$...$ &$b + \rhoRh\left(s, \left(1, \left| \mAb \right|\right)\right) + \Suh$\\ \hline
$2$ &$-b + \rhoRh\left(s, \left(2, 1\right)\right) +  \Suh$ &? &$...$ &?\\ \hline
$...$ &$...$ &$...$ &$...$ &$...$\\ \hline
$\left| \mAa \right|$ &$-b + \rhoRh\left(s, \left(\left| \mAa \right|, 1\right)\right) +  \Suh$ &? &$...$ &?\\ \hline
\end{tabular} \end{center}
For $\left(1, 1\right)$ to be the $\iota$ strict, thus unique, Nash equilibrium for all $Q \in \left[\Ql, \Qu\right]$, sufficient conditions are, for $a_{1} \neq 1$ and $a_{2} \neq 1$,
\begin{align}
- \rhoRh\left(s, \left(1, 1\right)\right) + \Slh - \dfrac{\iota}{2} &\geq - \dfrac{b}{2 H} \left(H - h + 1\right) \geq -b + \rhoRh\left(s, \left(a_{1}, 1\right)\right) + \Suh + \dfrac{\iota}{2} ,\nonumber
\\ \rhoRh\left(s, \left(1, 1\right)\right) + \Suh + \dfrac{\iota}{2} &\leq \dfrac{b}{2 H} \left(H - h + 1\right) \leq b - \rhoRh\left(s, \left(1, a_{2}\right)\right) + \Slh - \dfrac{\iota}{2} ,\nonumber
\end{align}
which would be true in period $1$ if the following is satisfied for $\textbf{a}$ such that either $a_{1} = \pidagha\left(s\right)$ or $a_{2} = \pidaghb\left(s\right)$,
\begin{align}
\rhoRh\left(s, \textbf{a}\right) &\leq \dfrac{b - \iota}{4 H} \leq \dfrac{b}{2 H} - \dfrac{\iota}{2,}\nonumber
\end{align}
which in turn implies,
\begin{align}
\Slh &\geq - \dfrac{b}{2 H} \left(H - h + 1\right) + \dfrac{b}{4 H},\nonumber
\\ \Suh &\leq \dfrac{b}{2 H} \left(H - h + 1\right) - \dfrac{b}{4 H}.\nonumber
\end{align}
We provide the formal proof below.

\begin{proof}  \label{proof:feaspf} 
We assume  is satisfied, meaning, for each $h \in \left[H\right], s \in \mS, \textbf{a} \in \mA$,
\begin{align}
\rhoRh\left(s, \textbf{a}\right) &\leq \dfrac{b - \iota}{4 H} \leq \dfrac{b}{2 H} - \dfrac{\iota}{2} . \label{eq:ccc}
\end{align}
In addition, take $R \in \mCR$, based on ~\eqref{eq:fsatk}, we can compute $\Rht$ using ~\eqref{eq:srhat}, and for each $h \in \left[H\right], s \in \mS$,
\begin{align}
- \rhoRh\left(s, \pidagh\left(s\right)\right) &\leq \Rh\left(s, \pidagh\left(s\right)\right) \leq \rhoRh\left(s, \pidagh\left(s\right)\right), \label{eq:rooul}
\\ -b - \rhoRh\left(s, \left(a_{1}, \pidaghb\left(s\right)\right)\right) &\leq \Rh\left(s, \left(a_{1}, \pidaghb\left(s\right)\right)\right)\nonumber
\\ &\leq -b + \rhoRh\left(s, \left(a_{1}, \pidaghb\left(s\right)\right)\right), \label{eq:raoul}
\\ b - \rhoRh\left(s, \left(\pidagha\left(s\right), a_{2}\right)\right) &\leq \Rh\left(s, \left(\pidagha\left(s\right), a_{2}\right)\right)\nonumber
\\ &\leq b + \rhoRh\left(s, \left(\pidagha\left(s\right), a_{2}\right)\right). \label{eq:robul}
\end{align}
We proceed by induction. In period $H$, for $a_{1} \neq \pidagHa\left(s\right)$,
\begin{align}
\QH^{\pidag}\left(s, \pidagH\left(s\right)\right) - \dfrac{\iota}{2} &= \RH\left(s, \pidagH\left(s\right)\right) - \dfrac{\iota}{2}\nonumber
\\ &\stackrel{~\eqref{eq:rooul}}{\geq} - \rhoRh\left(s, \pidagH\left(s\right)\right) - \dfrac{\iota}{2}\nonumber
\\ &\stackrel{~\eqref{eq:ccc}}{\geq} - \dfrac{b}{2 H} \label{eq:qluhb}
\\ &\geq -b + \dfrac{b}{2 H}\nonumber
\\ &\stackrel{~\eqref{eq:ccc}}{\geq} - b + \rhoRh\left(s, \left(a_{1}, \pidagHb\left(s\right)\right)\right) + \dfrac{\iota}{2}\nonumber
\\ &\stackrel{~\eqref{eq:raoul}}{\geq} \RH\left(s, \left(a_{1}, \pidagHb\left(s\right)\right)\right) + \dfrac{\iota}{2}\nonumber
\\ &= \Qh^{\pidag}\left(s, \left(a_{1}, \pidagHb\left(s\right)\right)\right) + \dfrac{\iota}{2} ,\nonumber
\end{align}
and for $a_{2} \neq \pidagHb\left(s\right)$,
\begin{align}
\QH^{\pidag}\left(s, \pidagH\left(s\right)\right) + \dfrac{\iota}{2} &= \RH\left(s, \pidagH\left(s\right)\right) + \dfrac{\iota}{2}\nonumber
\\ &\stackrel{~\eqref{eq:rooul}}{\leq} \rhoRh\left(s, \pidagH\left(s\right)\right) + \dfrac{\iota}{2}\nonumber
\\ &\stackrel{~\eqref{eq:ccc}}{\leq} \dfrac{b}{2 H} \label{eq:qluha}
\\ &\leq b - \dfrac{b}{2 H}\nonumber
\\ &\stackrel{~\eqref{eq:ccc}}{\leq} b - \rhoRh\left(s, \left(a_{1}, \pidagHb\left(s\right)\right)\right) - \dfrac{\iota}{2}\nonumber
\\ &\stackrel{~\eqref{eq:raoul}}{\leq} \RH\left(s, \left(\pidagHa\left(s\right), a_{2}\right)\right) - \dfrac{\iota}{2}\nonumber
\\ &= \QH^{\pidag}\left(s, \left(\pidagHa\left(s\right), a_{2}\right)\right) - \dfrac{\iota}{2} .\nonumber
\end{align}
Now, fix a period $h < H$, we assume in periods $h' \in \left\{h + 1, h + 2, ..., H\right\}$, in every state $s \in \mS, \pidag$ is the Nash equilibrium, and,
\begin{align}
- \dfrac{b}{2} \left(H - h' + 1\right) &\leq \Qhp^{\pidag}\left(s, \pidaghp\left(s\right)\right) \leq \dfrac{b}{2} \left(H - h' + 1\right). \label{eq:qhhul}
\end{align}
This is true in period $H$ due to ~\eqref{eq:qluhb} and ~\eqref{eq:qluha}.
\\* Now in period $h$, for a fixed $s \in \mS$, for any $a_{1} \neq \pidagha\left(s\right)$,
\begin{align}
\Qh^{\pidag} & \left(s, \pidagh\left(s\right)\right) - \dfrac{\iota}{2}\nonumber
\\ &= \Rh\left(s, \pidagh\left(s\right)\right) + \displaystyle\sum_{s' \in \mS} \Ph\left(s' | s, \pidagh\left(s\right)\right) \Qhh^{\pidag}\left(s', \pidaghh\left(s'\right)\right) - \dfrac{\iota}{2}\nonumber
\\ &\geq \Rh\left(s, \pidagh\left(s\right)\right) + \displaystyle\min_{s' \in \mS} \Qhh^{\pidag}\left(s', \pidaghh\left(s'\right)\right) - \dfrac{\iota}{2}\nonumber
\\ &\stackrel{~\eqref{eq:qhhul}}{\geq} \Rh\left(s, \pidagh\left(s\right)\right) - \dfrac{b}{2} \left(H - h\right) - \dfrac{\iota}{2}\nonumber
\\ &\stackrel{~\eqref{eq:rooul}}{\geq} - \rhoRh\left(s, \pidagh\left(s\right)\right) - \dfrac{b}{2 H} \left(H - h\right) - \dfrac{\iota}{2}\nonumber
\\ &\stackrel{~\eqref{eq:ccc}}{\geq} - \dfrac{b}{2 H} - \dfrac{b}{2 H} \left(H - h\right)\nonumber
\\ &\geq - \dfrac{b}{2 H} \left(H - h + 1\right) \label{eq:qlubb}
\\ &\geq -b + \dfrac{b}{2 H} + \dfrac{b}{2 H} \left(H - h\right)\nonumber
\\ &\stackrel{~\eqref{eq:ccc}}{\geq} -b + \rhoRh\left(s, \left(a_{1}, \pidaghb\left(s\right)\right)\right) + \dfrac{b}{2 H} \left(H - h\right) + \dfrac{\iota}{2}\nonumber
\\ &\stackrel{~\eqref{eq:raoul}}{\geq} \Rh\left(s, \left(a_{1}, \pidaghb\left(s\right)\right)\right) + \dfrac{b}{2 H} \left(H - h\right) + \dfrac{\iota}{2}\nonumber
\\ &\stackrel{~\eqref{eq:qhhul}}{\geq} \Rh\left(s, \left(a_{1}, \pidaghb\left(s\right)\right)\right) + \displaystyle\max_{s' \in \mS} \Qhh^{\pidag}\left(s', \left(a_{1}, \pidaghh\left(s'\right)\right)\right) + \dfrac{\iota}{2}\nonumber
\\ &\geq \Rh\left(s, \left(a_{1}, \pidaghb\left(s\right)\right)\right) + \displaystyle\sum_{s' \in \mS} \Ph\left(s' | s, \left(a_{1}, \pidaghb\left(s\right)\right)\right) \Qhh^{\pidag}\left(s', \left(a_{1}, \pidaghh\left(s'\right)\right)\right) + \dfrac{\iota}{2}\nonumber
\\ &= \Qh^{\pidag}\left(s, \left(a_{1}, \pidaghb\left(s\right)\right)\right) + \dfrac{\iota}{2} ,\nonumber
\end{align}
and for $a_{2} \neq \pidaghb\left(s\right)$,
\begin{align}
\Qh^{\pidag} & \left(s, \pidagh\left(s\right)\right) + \dfrac{\iota}{2}\nonumber
\\ &= \Rh\left(s, \pidagh\left(s\right)\right) + \displaystyle\sum_{s' \in \mS} \Ph\left(s' | s, \pidagh\left(s\right)\right) \Qhh^{\pidag}\left(s', \pidaghh\left(s'\right)\right) + \dfrac{\iota}{2}\nonumber
\\ &\leq \Rh\left(s, \pidagh\left(s\right)\right) + \displaystyle\max_{s' \in \mS} \Qhh^{\pidag}\left(s', \pidaghh\left(s'\right)\right) + \dfrac{\iota}{2}\nonumber
\\ &\stackrel{~\eqref{eq:qhhul}}{\leq} \Rh\left(s, \pidagh\left(s\right)\right) + \dfrac{b}{2 H} \left(H - h\right) + \dfrac{\iota}{2}\nonumber
\\ &\stackrel{~\eqref{eq:rooul}}{\leq} \rhoRh\left(s, \pidagh\left(s\right)\right) + \dfrac{b}{2 H} \left(H - H\right) + \dfrac{\iota}{2}\nonumber
\\ &\stackrel{~\eqref{eq:ccc}}{\leq} \dfrac{b}{2 H} + \dfrac{b}{2 H} \left(H - h\right)\nonumber
\\ &= \dfrac{b}{2 H} \left(H - h + 1\right) \label{eq:qluaa}
\\ &\leq b - \dfrac{b}{2 H} - \dfrac{b}{2 H} \left(H - h\right)\nonumber
\\ &\stackrel{~\eqref{eq:ccc}}{\leq} b + \rhoRh\left(s, \left(a_{1}, \pidaghb\left(s\right)\right)\right) - \dfrac{b}{2 H} \left(H - h\right) - \dfrac{\iota}{2}\nonumber
\\ &\stackrel{~\eqref{eq:raoul}}{\leq} \Rh\left(s, \left(\pidagha\left(s\right), a_{2}\right)\right) - \dfrac{b}{2 H} \left(H - h\right) - \dfrac{\iota}{2}\nonumber
\\ &\stackrel{~\eqref{eq:qhhul}}{\leq} \Rh\left(s, \left(\pidagha\left(s\right), a_{2}\right)\right) + \displaystyle\min_{s' \in \mS} \Qhh^{\pidag}\left(s', \left(\pidagha\left(s\right), a_{2}\right)\right) - \dfrac{\iota}{2}\nonumber
\\ &\leq \Rh\left(s, \left(\pidagha\left(s\right), a_{2}\right)\right) + \displaystyle\sum_{s' \in \mS} \Ph\left(s' | s, \left(\pidagha\left(s\right), a_{2}\right)\right) \Qhh^{\pidag}\left(s', \left(\pidagha\left(s\right), a_{2}\right)\right) - \dfrac{\iota}{2}\nonumber
\\ &= \Qh^{\pidag}\left(s, \left(\pidagha\left(s\right), a_{2}\right)\right) - \dfrac{\iota}{2} .\nonumber
\end{align}
Therefore, $\pidag$ is the Nash equilibrium in period $h$ state $s$, and ~\eqref{eq:qlubb} and ~\eqref{eq:qluaa} are consistent ~\eqref{eq:qhhul}. By induction, $\pidag$ is a strict, thus unique, Nash equilibrium in every stage game, making $\pidag$ the unique MPE.

\end{proof}

\subsection{Code Details}

We conducted our experiments using standard python3 libraries. The only exception being we used the gurobi LP solver. We provide our code in a jupyter notebook with an associated database file so that our experiments can be easily reproduced. The notebook already reads in the database by default so no file management is needed. Simply ensure the notebook is in the same directory as the database folder.
